# Supplementary material for: QUTCC: Quantile Uncertainty Training and Conformal Calibration for Imaging Inverse Problems
Source: arXiv:2507.14760 source file (2026-11-17)
Supplement: Supplementary file 1 [file Quantile_Crossing_QUTCC_Im2Im.tex]

\sisetup{
  scientific-notation=true,
  exponent-product=\cdot,
  output-exponent-marker=\text{e},
  round-mode=figures,
  round-precision=3,
  table-number-alignment = center,
  text-series-to-math = true,
    propagate-math-font = true
}

% \begin{table}[h!]
% \centering
% \resizebox{0.8\textwidth}{!}{%
% \begin{tabular}{l S[scientific-notation=true] S[scientific-notation=true] S}
% \toprule
% \textbf{Task} & \textbf{Crossed Pixels} & \textbf{Total Pixels} & \textbf{\% Crossing} \\
% \midrule
% QPI       & 0      & 3.2768e7     & 0 \\
% Lenseless & 43478  & 2.359296e8   & 0.01842837863 \\
% MRI       & 22     & 2.9261824e9  & 0.0000007518328317 \\
% Gaussian Denoising & 111855 & 2097152000 & 0.005333662033 \\
% \bottomrule
% \end{tabular}
% }
% \caption{Quantile crossing statistics across modalities.}
% \end{table}


% ------------- TYLER RESULTS -------------

% \begin{table}[h!]
% \centering
% \resizebox{0.8\textwidth}{!}{%
% \begin{tabular}{l S[scientific-notation=true] S[scientific-notation=true] S}
% \toprule
% \textbf{Task} & \textbf{Crossed Pixels} & \textbf{Total Pixels} & \textbf{\% Crossing} \\
% \midrule
% QPI       & 0      & 676560896     & 0 \\
% MRI       & 21     & 11059200  & 0.000189887153 \\
% Gaussian Denoising & 22869 & 65536000 & 0.03489532470703125 \\
% Poisson Denoising & 0 & 52428800 & 0 \\

% \bottomrule
% \end{tabular}
% }
% \caption{Im2Im-UQ crossing statistics across modalities.}
% \end{table}

% \begin{table}[h!]
% \centering
% \resizebox{0.8\textwidth}{!}{%
% \begin{tabular}{l S[scientific-notation=true] S[scientific-notation=true] S}
% \toprule
% \textbf{Task} & \textbf{Crossed Pixels} & \textbf{Total Pixels} & \textbf{\% Crossing} \\
% \midrule
% QPI       & 5397      & 676560896     & 0.000797710898 \\
% MRI       & 0     & 11059200  & 0 \\
% Gaussian Denoising & 131 & 65536000 & 0.000199890137 \\
% Poisson Denoising & 0 & 52428800 & 0 \\

% \bottomrule
% \end{tabular}
% }
% \caption{Quantile crossing statistics across modalities.}
% \end{table}


% \begin{table}[h!]
% \centering
% \resizebox{0.9\textwidth}{!}{%
% \begin{tabular}{ll S S S S}
% \toprule
% \textbf{Metric} & \textbf{Model} & \textbf{QPI} & \textbf{MRI} & \textbf{Gaussian} & \textbf{Poisson} \\
% \midrule
% \multirow{2}{*}{Crossed Pixels}
%   & Im2Im-UQ & 0 & 21 & 22869 & 0 \\
%   & QUTCC & 5397 & 0 & 131 & 0 \\
% \addlinespace
% \multirow{2}{*}{Total Pixels}
%   & Im2Im-UQ &  676560896 & 11059200 & 65536000 & 52428800 \\
%   & QUTCC &  676560896 & 11059200 & 65536000 & 52428800 \\
% \addlinespace
% \multirow{2}{*}{\% Crossing}
%   & Im2Im-UQ & 0 & 0.000189887153 & 0.03489532470703125 & 0 \\
%   & QUTCC & 0.000797710898 & 0 & 0.000199890137 & 0 \\
% \bottomrule

% \end{tabular}%
% }
% \caption{Im2Im-UQ and quantile crossing statistics across modalities. }
% \end{table}



% \begin{table}[h!]
% \centering
% \resizebox{0.6\textwidth}{!}{%
% \begin{tabular}{ll S S S}
% \toprule
% \textbf{Dataset} & \textbf{Model} & \textbf{Crossed Pixels} & \textbf{Total Pixels} & \textbf{\% Crossing} \\
% \midrule
% \multirow{2}{*}{QPI}
%       & Im2Im-UQ &    0 &  676560896 & \textbf{0}              \\
%       & QUTCC & 5397 &  676560896 & 0.000797710898  \\
% \addlinespace
% \multirow{2}{*}{MRI}
%       & Im2Im-UQ &   21 &   11059200 & 0.000189887153  \\
%       & QUTCC &    0 &   11059200 & \textbf{0}               \\
% \addlinespace
% \multirow{2}{*}{Gaussian}
%  & Im2Im-UQ & 22869 &   65536000 & 0.03489532470703125 \\
%  & QUTCC &   131 &   65536000 & \textbf{0.000199890137}  \\
% \addlinespace
% \multirow{2}{*}{Poisson}
%   & Im2Im-UQ &    0 &   52428800 & \textbf{0}             \\
%   & QUTCC &    0 &   52428800 & \textbf{0}             \\
% \bottomrule
% \end{tabular}%
% }
% \caption{Quantile crossing statistics by dataset and model.}
% \end{table}

\begin{wraptable}{r}{8.5cm}
\centering
\resizebox{0.55\textwidth}{!}{%
\begin{tabular}{ll S S S}
\toprule
\textbf{Dataset} & \textbf{Model} & \textbf{Crossed Pixels} & \textbf{Total Pixels} & \textbf{\% Crossing} \\
\midrule
\multirow{2}{*}{QPI}
      & Im2Im-UQ &    \num{0} &  \num{676560896} & \textbf{\num{0}}              \\
      & QUTCC & \num{5397} &  \num{676560896} & \num{0.000797710898}  \\
\addlinespace
\multirow{2}{*}{MRI}
      & Im2Im-UQ &   \num{21} &   \num{11059200} & \num{0.000189887153}  \\
      & QUTCC &    \num{0} &   \num{11059200} & \textbf{\num{0}}               \\
\addlinespace
\multirow{2}{*}{Gaussian}
 & Im2Im-UQ & \num{22869} &   \num{65536000} & \num{0.03489532470703125} \\
 & QUTCC &   \num{131} &   \num{65536000} & \textbf{\num{0.000199890137}}  \\
\addlinespace
\multirow{2}{*}{Poisson}
  & Im2Im-UQ & \num{0} &   \num{52428800} & \textbf{\num{0}}             \\
  & QUTCC & \num{0} &   \num{52428800} & \textbf{\num{0}}             \\
\bottomrule
\end{tabular}%
}
\caption{Quantile crossing statistics by dataset and model.}
\end{wraptable}
